# Supplementary material for: Confidently Comparing Estimators with the c-value
Source: arXiv:2102.09705 source file (2022-12-19)
Supplement: Supplementary file 1 [file hierarchical_regression_supp.tex]

\section{Hierarchical Linear Regression}\label{sec:hierarchical_regression_supp}
In this section we demonstrate how one can apply our methodology to assess whether a hierarchical approach to regression 
utilizing data from a related response provides an improvement relative to independent analyses using ridge regression.
We provide details of this use-case, as well as results on several UCI datasets.
Despite sizeable improvements in predictions on held-out data, computed c-values fail to reliably confirm improved inferences.
We suspect this owes to the looseness of the evaluated bounds, resulting from poor conditioning of the design matrices in the problems we considered.

\subsection{Hierarchical regression details}
Consider fitting a linear model to a collection of $M$ pairs of covariates and responses, $\{\bar X_m, \bar Y_m\}_{m=1}^M$,
in order to make predictions of on collection of $N$ test points $\{X_n\}_{n=1}^N$ for which responses have not be observed, where each $\bar X_m$ and $X_n$ are vectors of $D$ covariates and each $\bar Y_m\in \R$. 
We model each response $m$ as independently, normally distributed about a linear function of the covariates,
$$
\bar Y_m \overset{indep}{\sim} \mathcal{N}(\bar X_m^\top \beta, 1),
$$
where $\beta \in \R^D$ is a vector of unknown covariate effects,
and desire to predict each unobserved test response $n$ as $X_n^\top \beta$.
With $\beta$ unknown, a standard approach is to estimate it by least squares.
In particular, collecting together the train and test data as $\bar X =[\bar X_1, \bar X_2, \dots, \bar X_M]^\top$,
$\bar Y = [\bar Y_1, \bar Y_2, \dots, \bar Y_M]^\top$ and
$X =[X_1, X_2, \dots, X_N]^\top$, where $\bar X \in \R^{M,D}, \bar Y \in \R^{M}$ and $X \in \R^{N,D}$,
we may write the least squares estimate as 
$$
\hat \beta := [ \bar X^\top \bar X ] \inv \bar X^\top \bar Y.
$$

Denoting our estimand by $\theta := X \beta,$ the associated maximum likelihood estimate is then $\hat \theta := X \hat \beta$,
which is distributed as 
$$
\hat \theta \sim \mathcal{N}(\theta, X(\bar X^\top \bar X)\inv X^\top ).
$$

However, when the data are noisy or sample sizes are small we may wonder if we can improve upon $\hat \theta$ by taking a Bayesian approach and modeling these data jointly with another dataset, and estimating $\theta$ instead by its posterior mean conditioned on both datasets.
In particular, imagine we have a second dataset of $L$ data points $\{W_l, Z_l\}_{l=1}^L$ where each $W_l \in \R^D$ and $Z_l\in \R$, and assume 
$$
Z_l \overset{indep}{\sim} \mathcal{N}(W_l^\top \eta, 1),
$$
where $\eta\in \R^D$ is an unknown parameter associated with the second dataset.

If we believe that the linear relationships are similar in these two datasets, we can reflect this in the prior of a hierarchical Bayesian model as
\(
\mu &\sim p(\mu) \propto 1,\\
\eta &\sim \mathcal{N}(\mu, \sigma_\beta^2 I_D),\\
\beta &\sim \mathcal{N}(\mu, \sigma_\beta^2 I_D)
\)
where $\sigma_\beta^2$ reflects how different we believe the parameters might be.
Conditional on $Z$, we then have
$$
\beta | Z \sim \mathcal{N}(\hat \eta, \Sigma_\beta)
$$
where $\hat \eta = (W^\top W)\inv W^\top Z$ is the least squares estimate of $\eta$ and 
the conditional variance is $\Sigma_\beta = 2\sigma_\beta^2 I_D + (W^\top W)\inv$,
which may be computed with standard Gaussian conjugacy calculations.
With some algebra, the posterior mean of $\theta$ may then be seen to be
\(
\theta^* &:=   \E[X \beta | Z, \bar Y] \\
%&= X \left[ \bar X^\top \bar X +  \Sigma_\beta\inv\right]\inv 
%\left[ \bar X\top \bar X \hat \beta + \Sigma_\beta\inv \hat \eta\right]\\
%&= X \left[I_D  +  (\bar X^\top \bar X)\inv   \Sigma_\beta\inv\right]\inv \hat \beta 
%+ X\left[ I_D + \Sigma_\beta \bar X^\top \bar X \right]\inv \hat \eta\\
%&= X \hat \beta -  X\left[I_D  +  \Sigma_\beta \bar X^\top \bar X \right]\inv \hat \beta 
%+X\left[ I_D + \Sigma_\beta \bar X^\top \bar X \right]\inv \hat \eta \\
%&= X \hat \beta -  X\left[I_D  +  \Sigma_\beta \bar X^\top \bar X \right]\inv (X^\top X) \inv X^\top X\hat \beta 
%+X\left[ I_D + \Sigma_\beta \bar X^\top \bar X \right]\inv \hat \eta \\
&= \hat \theta-  \left(X\left[I_D  +  \Sigma_\beta \bar X^\top \bar X \right]\inv X^\dagger \hat \theta
-X\left[ I_D + \Sigma_\beta \bar X^\top \bar X \right]\inv \hat \eta \right)
\)
where $X^\dagger=(X^\top X)\inv X^\top$ is the pseudo-inverse of $X$.
This is in precisely the form required to apply \Cref{eqn:affine_bya} (take $A=I_D$, $k=0$, $C=I_D-X\left[I_D  +  \Sigma_\beta \bar X^\top \bar X \right]\inv X^\dagger$
and $\ell=-X\left[ I_D + \Sigma_\beta \bar X^\top \bar X \right]\inv \hat \eta$).

\textbf{Results on Hierarchical Regression}
We show results for hierarchical regression in \Cref{table:h_regression} on three UCI datasets \citep{dua2019uci}.
To explore the ability to detect an improvement with additional data, we used as the additional dataset a random held-out subset of the original dataset.
For all datasets, all covariates and responses were standardized to have mean zero and variance one.
For the computer virus and crime datasets, the design matrices were sparse and extremely poorly conditioned,
so we replaced the design matrices with the top principle components.
The number of principle components was chosen so that $99.99$\% of the variance in the design was explained.
For each dataset, we chose the size of the auxiliary dataset $L$ to be much larger than that of the training set $M$,
so that it would be more likely to lead to a detectable improvement.

To choose the prior variance, we first estimated the variance of the noise by
$$
\hat \sigma_{obs}^2  := \|P_X^\perp Y\|^2 / (N-D),
$$
which in the case of correct model specification is unbiased and independent of $\hat \beta$.
We then choose 
$$
\sigma_\beta^2 = \frac{1}{2}(1-\hat \sigma_{obs}^2 )/D.
$$
This choice is consistent with the idea that half of the variance in $Y$ associated with the covariates
is independent across the two datasets.

\begin{table}[h!]
\centering
\begin{tabular}{||c c c c c c c c||} 
\hline
    Dataset & D & L & M & N & b(y,0.9) & c-value & Win  \\ [0.5ex]
\hline
    Year & 91 & 5,000 & 500 & 5,000 & 0.037 & 0.945 & 0.18 \\  
    Computer Virus& 62 & 50,000 & 10,000 & 10,000 & -788.6 & 0.000 & 449.9 \\ 
    Crime Prediction & 70 & 1,000 & 500 & 715 & -0.17 & 0.600  & 0.08 \\ [1ex] 
\hline
\end{tabular}
    \caption{C-values for evaluating Bayes estimates from hierarchical linear models on three UCI datasets.}\label{table:h_regression}
\end{table}

We report a summary of these dataset and our results in \Cref{table:h_regression}.
Interestingly, though prediction performance on a held-out set is improved with the hierarchical model in all cases, none of these analyses provide significant c-values.
We hypothesize that this is due in part to the looseness of our bounds for this application.
